# Supplementary material for: Dependent Inductive and Coinductive Types are Fibrational Dialgebras
Source: arXiv:1508.06779 source file (2015-09-10)
Supplement: Supplementary file 1 [file appendix.tex]

\section{Proofs  \secRef{construct-dt}}
\label{app:proofs-construct-dt}

We need the following technical tool.
\begin{lemma}[Primitive corecursion]
  Let $\Cat{C}$ be a category with binary coproducts and $\Endo{F}{\Cat{C}}$ an
  endofunctor on $\Cat{C}$ with a final coalgebra $(M, \xi : M \to FM)$.
  For every morphism $c : X \to F(X + M)$ in $\Cat{C}$, there is a
  unique map $h : X + M \to M$, such that $h \circ \kappa_2 = \id_M$ and the
  following diagram commutes.
  \begin{equation*}
    \begin{tikzcd}[column sep = 3em]
      X \dar{c} \rar{h \, \circ \, \kappa_1} & M \dar{\xi} \\
      F(X + M) \rar{F h} & FM
    \end{tikzcd}
  \end{equation*}
\end{lemma}
\begin{proof}
  We define $h$ as the coinductive extension as in the following diagram.
  \begin{equation*}
    \begin{tikzcd}[column sep = 3em]
      X \dar{c} \rar{\kappa_1}
      & X + M \rar{h} \dar{\coprodArr{c, F \kappa_2 \circ \xi}}
      & M \dar{\xi} \\
      F(X + M) \rar[equal]{}
      & F(X + M) \rar{F h}
      & FM
    \end{tikzcd}
  \end{equation*}
  It is easily checked that the rectangle on the right commutes if and
  only if the above identities hold.
  Thus uniqueness of $h$ follows from uniqueness of coinductive extensions.
\end{proof}

Primitive corecursion allows us to define one-step behaviour as follows.
\begin{lemma}[One-step extension]
  Let $F$ and $(M, \xi)$ as above, and let $f : M \to FM$ be a morphism.
  Then there exists a unique $g : M \to M$, such that
  $\xi \circ g = f$.
\end{lemma}
\begin{proof}
  We define $g = h \circ \kappa_1$, where $h$ arises by primitive corecursion
  of $F \kappa_2 \circ f$.
  It is then straightforward to show that $\xi \circ g = f$ if and only
  the identities of primitive corecursion hold.
  Thus $g$ is the unique morphism for which this identity holds.
\end{proof}

Using the definition of $V$ as equaliser of $u_1$ and $u_2$, we can
characterise elements of $V$ as follows.
First we note that $V$ is indexed over $I$ by
$q = V \xrightarrow{g} M_f \xrightarrow{\rho} A \xrightarrow{t} I$,
where $\rho$ is the root map given by composing $\xi_f$ with projection
for coproducts.
Abusing notation, we will use $V$ instead of $q$, and write $x : V_i$ if
$x : V$ and $q \, x = i$.

Let $X$ be an object in $\BCat$.
An object $R \in \slice{\BCat}{X^2}$ is called a relation, and we say that
elements $x, y : X$ are related by are, denoted $(x, y) : R$, if there is
a $z : R$, such that $\pi_1 (R \, z) = x$ and $\pi_2 (R \, z) = y$.
\begin{lemma}[Internal bisimulations]
  Let $f : B \to A$ be a polynomial and $R \in \slice{\BCat}{M_f^2}$ a relation
  over $M_f$ such that
  \begin{align*}
    \forall (x_1, x_2) : R.
    & \text{ if } \xi_f (x_k) = (a_k, v_k) \\
    & \text{ then } a_1 = a_2 = a \\
    & \text{ and } (\forall b : B. f b = a \Rightarrow (v_1 \, b, v_2 \, b) : R).
  \end{align*}
  Then for all $(x_1, x_2) : R$, we have that $x_1 = x_2$.
\end{lemma}
\begin{proof}
  It is easy to see that this allows us to define a coalgebra
  structure on $R : U \to M_f^2$ such that $\pi_k \circ R : U \to M_2$ are
  homomorphism for $k = 1, 2$, which implies by finality of $M_f$ that
  $\pi_1 \circ R = \pi_2 \circ R$.
\end{proof}

In the following lemmas we use the notation introduced in the proof of
\iThmRef{dep-final-coalg-from-non-dep}.
\begin{lemma}
  \label{lem:phi-u1-eq-gives-index-and-elem-V}
  If $y : M_f$ and $b : B$ such that $\phi (u_1 \, y, b) = u_1 \, y$,
  then $q \, y = s \, b$ and $u_1 \, y = u_2 \, y$.
\end{lemma}
\begin{proof}
  We let $\xi_f \, y = (a, v)$ and then find that
  \begin{align*}
    \xi_{f \times I} \, (\phi (u_1 \, y, b))
    & = (a, s \, b, \lambda b'. \phi (u_1 \, (v \, b'), b')) \\
    & = (a, t \, a, \lambda b'. u_1 \, (v \, b')) & \text{ by assumption} \\
    & = \xi_{f \times I} \, (u_1 \, y).
  \end{align*}
  Thus $s \, b = t \, a = q \, y$ and
  $\phi (u_1 \, (v \, b'), b') = u_1 \, (v \, b')$ for all
  $b' : B$ with $f \, b = a$.
  This gives us
  \begin{align*}
    \xi_{f \times I} \, (u_1 \, y)
    & = (a, t \, a, \lambda b'. u_1 \, (v \, b')) \\
    & = (a, t \, a, \lambda b'. \phi (u_1 \, (v \, b'), b'))
    & \text{ see above} \\
    & = \xi_{f \times I} \, (u_2 \, y)
  \end{align*}
  as required.
\end{proof}

\begin{lemma}
  \label{lem:characterisation-V}
  Let $i : I$ and $x : M_f$, then the following are equivalent
  \begin{enumerate}
  \item \label{characterisation-V:x-in-Vi}
    $x : V_i$
  \item \label{characterisation-V:x-in-Vi-def}
    $u_1 \, x = u_2 \, x \text{ and } q \, x = i$
  \item \label{characterisation-V:x-in-Vi-coinductive}
    $ \xi_f \, x = (a : A , v : \Pi_f M_f), \, t \, a = i \text{ and }
    (\forall b : B. f \, b = a \Rightarrow v \, b : V_{s \, b})$
  \item \label{characterisation-V:x-in-Vi-poly-type}
    $\xi_f \, x = (a : A , v : \Pi_f M_f), \, t \, a = i \text{ and }
    v : \Pi_f (\reidx{s} V)$
  \end{enumerate}
\end{lemma}
\begin{proof}
  The equivalences \ref{characterisation-V:x-in-Vi} $\iff$
  \ref{characterisation-V:x-in-Vi-def}
  and \ref{characterisation-V:x-in-Vi-coinductive} $\iff$
  \ref{characterisation-V:x-in-Vi-poly-type}
  are the definitions, so let us prove \ref{characterisation-V:x-in-Vi-def}
  $\iff$ \ref{characterisation-V:x-in-Vi-coinductive}.
  % Note that \ref{characterisation-V:x-in-Vi-coinductive} defines a coinductive
  % predicate on $M_f$, so we will use coinduction to prove it.

  We begin by proving \ref{characterisation-V:x-in-Vi-def}
  $\Rightarrow$ \ref{characterisation-V:x-in-Vi-coinductive}.
  Let $x : M_f$ with $u_1 \, x = u_2 \, x$ and $q \, x = i$.
  Then we have for $x_f \, x = (a, v)$ that $t \, a = q \, x = i$,
  \begin{equation*}
    \xi_{f \times I} \, (u_1 \, x)
    = \polySem{f \times I} (u_1) \, (p_{M_f} \, (\xi_f \, x))
    = (a, t \, a, \lambda b. u_1 (v \, b))
  \end{equation*}
  and
  \begin{align*}
    \xi_{f \times I} \, (u_2 \, x)
    & = \polySem{f \times I}(\phi) \,
        (\Sigma_{A \times I} K \, (\xi_{f \times I} \, (u_1 \, x))) \\
    & = \polySem{f \times I}(\phi) \,
        (\Sigma_{A \times I} K \, (a, t \, a, \lambda b. u_1 \, (v \, b)) \\
    & = (a, t \, a, \lambda b. \phi( u_1 \, (v \, b), b)).
  \end{align*}
  By these calculations and Since $u_1 \, x = u_2 \, x$, we also have
  for all $b : B$ with $f \, b = a$ that
  $u_1 (v \, b) = \phi( u_1 \, (v \, b), b)$.
  Applying \iLemRef{phi-u1-eq-gives-index-and-elem-V} to $y = v \, b$ we get
  that $q \, (v \, b) = s \, b$ and
  $u_1 \, (v \, b) = u_2 \, (v \, b)$, thus $v \, b : V_{s \, b}$ and
  \ref{characterisation-V:x-in-Vi-coinductive} holds.

  For the other direction, assume that
  $ \xi_f \, x = (a : A , v : \Pi_f M_f), \, t \, a = i \text{ and }
  (\forall b : B. f \, b = a \Rightarrow v \, b : V_{s \, b})$.
  We show that $u_1 \, x = u_2 \, x$ by giving a bisimulation $R$ that relates
  $u_1 \, x $ and $u_2 \, x$.
  We put
  \begin{align*}
    & X = \T + \Sigma_B. \reidx{s} V \\
    & R : X \to M_f \times M_f \\
    & R (\ast) = (u_1 \, x, u_2 \, x) \\
    & R (b, y) = (u_1 \, y, \phi (y, b))
  \end{align*}
  which is a relation over $M_f$.
  To prove that $R$ is a bisimulation, there are two cases to consider.
  First, we have $(u_1 \, x, u_2 \, x) : R$.
  Note that
  \begin{align*}
    \xi_{f \times I} \, (u_1 \, x)
    & = (a, t \, a, \lambda b. u_1 \, (v \, b))
    \intertext{and}
    \xi_{f \times I} \, (u_2 \, x)
    & = (a, t \, a, \lambda b. \phi (u_1 \, (v \, b), b))
  \end{align*}
  so that
  $\rho_{f \times I} \, (u_1 \, x) = (a, t \, a) = \rho_{f \times I} (u_1 \, x)$.
  Moreover, we have for all $b : B$ that $u_1 \, (v \, b)$ and
  $\phi (u_1 \, (v \, b), b)$ are related by $R$.
  For the second case, let $b : B$ and $y : V_{s \, b}$.
  Then for $x_f y = (a', v')$ we have
  \begin{align*}
    \xi_{f \times I} \, (u_1 \, y)
    & = (a', t \, a', \lambda b'. u_1 \, (v' \, b'))
    \intertext{and}
    \xi_{f \times I} \, \phi (y, b)
    & = (a', s \, b, \lambda b'. \phi (u_1 \, (v' \, b'), b')).
  \end{align*}
  Since $y : V_{s \, b}$, we have, by definition, that
  $s \, b = q \, y = t \, a'$, thus $(a', t \, a') = (a', s \, b)$.
  Moreover, $u_1 \, (v' \, b')$ and $u_1 (v' \, b', b')$ are again related by
  $R$.
  Hence, we can conclude that $R$ is a bisimulation, and so
  $u_1 \, x = u_2 \, x$.
\end{proof}
